# Supplementary material for: Quantum perturbation theory using Tensor cores and a deep neural network
Source: arXiv:2203.09621 ancillary file (2022-05-10)
Supplement: Supplementary file 1 [file SI.pdf]

# I. SUPPLEMENTAL INFORMATION

The following is a Python implementation of the DNN-SP2-PT method using an example Hamiltonian and an example perturbation. This Python script is a translation of the pseudocode in Alg. 1 to Alg. 3.

```
import numpy as np

def UPDATE_LAYER_0(X0,S0,TrS0,D0_converged,v_sigma,\
                   idemp_err,layer,frob_err_0):

    M=0

    #### CONVERGENCE TEST FOR S0 USING S0 CONVERGENCE CRITERIA
    if (idemp_err[layer] <= 0):
        D0_converged = True
        print("===================")
        print("S0 converged to D0.")
        print("===================")
        frob_err_0 = np.linalg.norm(S0-X0)
        M = layer
    elif (layer > 2 and v_sigma[layer-1] != v_sigma[layer-2]\
         and idemp_err[layer] >= 4.5 * idemp_err[layer-2] * idemp_err[layer-2]):
        D0_converged = True
        print("===================")
        print("S0 converged to D0.")
        print("===================")
        frob_err_0 = np.linalg.norm(S0-X0)
        M = layer

    else:
        #### UPDATE S0 IF IT HAS NOT CONVERGED
        sigma = v_sigma[layer]
        W = sigma                           # Weight function
        B = (1-sigma)*S0                    # Bias function
        S0 = W*X0 + B                       # Apply weight and bias

        TrS0 = W*TrX0 + (1-sigma)*TrS0      # Update occupation

    return S0, TrS0, D0_converged, M, frob_err_0

def UPDATE_LAYER_1(X1,S1,sigma,D0_converged,D1_converged,\
                   frob_err_0,frob_err_1,idemp_err,layer,M):

    #### CONVERGENCE TEST FOR S1 ONLY AFTER S0 CONVERGES
    if (D0_converged==True):

        #### CONVERGENCE CRITERIA FOR S1
        if (frob_err_1[layer] > 9 * frob_err_1[layer-2] * frob_err_0) \
            and (layer > M + 1):

            D1_converged=True
            print("===================")
            print("S1 converged to D1.")
            print("===================")

    #### UPDATE S1 IF IT HAS NOT CONVERGED
    if (D1_converged==False):
```

```
        W = sigma                         # Weight function
        B = (1-sigma)*S1                  # Bias function
        S1 = W*X1 + (1-W)*S1              # Apply weight and bias

    return S1, D1_converged

def generate_H(N):

    #### INITIALIZE SYMMETRIC TEST HAMILTONIAN
    H=np.zeros((N,N))

    for i in range(0,N):
        for j in range(i,N):
            H[i,j] = np.exp(-.5*np.abs(i-j))*np.sin(i+1);
            H[j,i] = H[i,j];

    return H

def generate_H1(N):

    #### INITIALIZE SYMMETRIC TEST PERTURBATION
    H1 = np.zeros((N,N))

    for i in range(0,N):
        for j in range(i,N):
            H1[i,j] = np.exp(-2*np.abs(i-j))*np.sin(3*i+1)/(i+1);
            H1[j,i] = H1[i,j];

    return H1


def gersgorin(M):

    #### FIND EIGENVALUE ESTIMATES USING THE GERSGORIN CIRCLE THEOREM
    min_e=0
    max_e=0

    for i in range(0,np.shape(M)[0]):

        #### EVALUE CIRCLE CENTER
        e=M[i,i]
        r=0

        #### SUM OF ABS VALUE OF COMPONENTS IN ROW I
        for j in range(0,np.shape(M)[0]):
           r+=np.abs(M[i,j])

        #### GERSGORIN EVALUE CIRCLE RADIUS
        r-=np.abs(e)

        #### UPDATE MIN AND MAX EVALUES AS YOU LOOPS OVER ROWS
        if e-r < min_e:
            min_e = e-r
        elif e+r > max_e:
            max_e = e+r

    return (min_e,max_e)
```

```
#### DNN FORMULATION OF DENSITY MATRIX PERTURBATION THEORY
if __name__=="__main__":                # Execute only when called from
                                        # command line

    #### PRINT 15 DIGITS
    np.set_printoptions(precision=15)

    #### INITIALIZE
    N = 1200                            # Number of basis orbitals
    Nocc = int(N*0.66)                  # Number of occupied orbitals
    eps = 1e-16                         # Small finite value in FP32
    sigma = 0                           # Initial value of sgn
    I = np.eye(N)                       # Identity matrix
    maxlayer = 200                      # Maximum number of layers
    v_sigma = np.zeros(maxlayer)        # Vector to record sigma
    idemp_err = np.zeros(maxlayer)      # Zeroth-order Idemp. error estimate
    frob_err_0 = 0                      # Frobenius norm of S0 Idemp. error
    frob_err_1 = np.zeros(maxlayer)     # Frobenius norm of S1 Idemp. error
    layer = 0                           # Deep layer counter
    M = 0                               # Layer where S0 converges to D0

    #### LOAD/CONSTRUCT HAMILTONIAN AS INPUT LAYER
    H0 = generate_H(N)                  # Symmetric NxN Hamiltonian matrix
    X0 = H0                             # Initial input layer
    H1 = generate_H1(N)                 # Perturbation
    X1 = H1                             # Initial input layer

    #### INITIAL IN-PLACE LEARNING FOR FIRST LAYER
    (hN,h1) = gersgorin(X0)             # Obtain eigenvalue estimates
                                        # using Gersgorin circle theorem

    #### INITIAL LINEAR TRANSFORM
    W0 = -1/(hN-h1)                     # Weight (scalar)
    B0 = (hN/(hN-h1))*I                 # Bias (diagonal matrix)
    S0 = W0*X0 + B0                     # Zeroth-order initial transform
    S0 = np.single(S0)                  # Store in FP32
    TrS0 = np.trace(S0)                 # Keep track of occupation

    S1 = W0*X1                          # First-order initial transform
    S1 = np.single(S1)                  # Store in single precision

    #### SET CONVERGENCE FLAGS
    D0_converged=False
    D1_converged=False


    #### COMPUTATIONAL DEEP LAYERS
    while D0_converged==False or D1_converged==False:

        #### ACTIVATION FUNCTION f^(1) FROM THREE DUAL
        #### HALF-PRECISION MATRIX-MATRIX MULTIPLICATIONS
        if D0_converged==False:
            X0_h = np.single(np.half(S0))            # FP16[S0], FP32 acc.
            X0_l = np.single(np.half(S0-X0_h))       # FP16[S0-X0_h], FP32 acc.
```

```
        X1_h = np.single(np.half(S1))               # FP16[S1], FP32 acc.
        X1_l = np.single(np.half(S1-X1_h))          # FP16[S1-X1_h], FP32 acc.
        X0X1_hh = np.single(np.matmul(X0_h,X1_h))   # FP16 mult., FP32 acc.
        X0X1_hl = np.single(np.matmul(X0_h,X1_l))   # FP16 mult., FP32 acc.
        X0X1_lh = np.single(np.matmul(X0_l,X1_h))   # FP16 mult., FP32 acc.
        X0X1 = np.single(X0X1_hh+X0X1_hl+X0X1_lh)   # Accumulation in FP32
        X1X0 = np.transpose(X0X1)                   # Use symmetry of S0 and S1
        X1 = np.single(X0X1 + X1X0)

        if D0_converged==False:

            #### ACTIVATION FUNCTION f^(0) FROM TWO DUAL
            #### HALF-PRECISION MATRIX-MATRIX MULTIPLICATIONS
            X0_hh = np.single(np.matmul(X0_h,X0_h)) # FP16 mult., FP32 acc.
            X0_hl = np.single(np.matmul(X0_h,X0_l)) # FP16 mult., FP32 acc.
            X0_lh = np.transpose(X0_hl)             # Use symmetry of S0
            X0 = np.single(X0_hh+X0_hl+X0_lh)       # Accumulation in FP32

            TrX0 = np.trace(X0)                     # Approx. occupation

            #### ZEROTH ORDER IDEMPOTENCY ERROR ESTIMATE
            idemp_err[layer] = TrS0-TrX0
            print("Layer␣=␣" + str(layer) + ",␣Error␣=␣" + str(idemp_err[layer]))

            #### LEARNING THROUGH BINARY ON-THE-FLY
            #### IN-PLACE OCCUPATION ERROR MINIMIZATION
            sigma = np.sign(np.abs(2*TrS0 - TrX0 - Nocc) \
                               - np.abs(TrX0 - Nocc) + eps)


            v_sigma[layer] = sigma


            #### UPDATE D0 APPROXIMATION AND CHECK CONVERGENCE
            (S0, TrS0, D0_converged, M, frob_err_0) \
            = UPDATE_LAYER_0(X0,S0,TrS0,D0_converged,\
                                 v_sigma,idemp_err,layer,frob_err_0)

        else:

            #### IF S0 HAS CONVERGED, DO NOT UPDATE S0 AND FLIP SIGMA
            S0 = S0
            sigma = (-1)*v_sigma[layer-1]           # Flip sigma
            v_sigma[layer] = sigma
            W = v_sigma[layer]                      # Weight function

        frob_err_1[layer] = np.linalg.norm(S1-X1)
        print("Frobenius␣error␣for␣S1␣=␣" + str(frob_err_1[layer]))


        #### UPDATE D1 APPROXIMATION AND CHECK CONVERGENCE
        (S1,D1_converged) \
        = UPDATE_LAYER_1(X1,S1,sigma,D0_converged, D1_converged,\
                              frob_err_0,frob_err_1,idemp_err,layer,M)

        #### UPDATE LAYER
        layer += 1
```

```
    D0 = np.double(S0)        # Output layer estimate of D^{(0)}
    D1 = np.double(S1)        # Output layer estimate of D^{(1)}
```
